# Supplementary material for: Multi-center decomposition of molecular densities: A numerical perspective
Source: arXiv:2405.08455 source file (2024-10-24)
Supplement: Supplementary file 1 [file supp.pdf]

Supporting Information for:

# Multi-center decomposition of molecular densities: A numerical perspective


YingXing Cheng,[†] Eric Cancès,[‡] Virginie Ehrlacher,[‡] Alston J. Misquitta,[¶] and Benjamin Stamm[*,†]

†*Institute of Applied Analysis and Numerical Simulation, University of Stuttgart, Pfaffenwaldring 57, 70569 Stuttgart, Germany*

‡*CERMICS, Ecole des Ponts and Inria Paris, 6 & 8 Avenue Blaise Pascal, 77455 Marne-la-Vallée, France*

¶*Queen Mary University of London, Mile End Road, London E1 4NS, United Kingdom*

E-mail: benjamin.stamm@mathematik.uni-stuttgart.de


## S1 The exponents and initial values for the Gaussian density basis

Table S1: The exponents for the Gaussian s-type density basis in both GISA and LISA methods in atomic units.

| k | H | C | N | O | F | Si | S | Cl | Br |
|---|---|---|---|---|---|---|---|---|---|
| 1 | 5.6720 | 148.3000 | 178.0000 | 220.1000 | 232.2846 | 366.5112 | 528.7272 | 622.3137 | 1027.3862 |
| 2 | 1.5050 | 42.1900 | 52.4200 | 65.6600 | 73.1726 | 104.3665 | 147.5558 | 180.7931 | 84.3671 |
| 3 | 0.5308 | 15.3300 | 19.8700 | 25.9800 | 30.0344 | 15.5123 | 17.6378 | 98.9482 | 67.8966 |
| 4 | 0.2204 | 6.1460 | 1.2760 | 1.6850 | 2.4199 | 9.5104 | 17.5077 | 69.1275 | 64.9399 |
| 5 | | 0.7846 | 0.6291 | 0.6860 | 1.0096 | 7.8724 | 15.1251 | 20.2219 | 30.7992 |
| 6 | | 0.2511 | 0.2857 | 0.2311 | 0.3263 | 5.3849 | 7.1494 | 8.9831 | 6.4459 |
| 7 | | | | | | 3.7020 | 0.5499 | 0.6418 | 5.3029 |
| 8 | | | | | | 0.3241 | 0.2713 | 0.3052 | 4.4950 |
| 9 | | | | | | 0.1076 | 0.1013 | 0.1370 | 2.6361 |
| 10 | | | | | | | | | 0.7183 |
| 11 | | | | | | | | | 0.3682 |
| 12 | | | | | | | | | 0.1390 |

Table S2: The initial values for the Gaussian s-type density basis in both GISA and LISA methods in atomic units.

| k | H | C | N | O | F | Si | S | Cl | Br |
|---|---|---|---|---|---|---|---|---|---|
| 1 | 0.0429 | 0.1330 | 0.1627 | 0.1869 | 0.2326 | 0.5063 | 0.4472 | 0.4127 | 1.4011 |
| 2 | 0.2639 | 0.5955 | 0.6567 | 0.6576 | 0.7623 | 1.1758 | 1.1959 | 1.1066 | 0.0001 |
| 3 | 0.4790 | 1.0749 | 0.9993 | 0.9751 | 0.8161 | 0.0001 | 0.0001 | 0.1210 | 0.0001 |
| 4 | 0.2127 | 0.0202 | 2.3257 | 3.0657 | 2.9602 | 1.7484 | 0.0001 | 0.0001 | 6.6184 |
| 5 | | 2.7117 | 1.8949 | 2.5622 | 3.3411 | 0.4014 | 1.4710 | 0.9133 | 0.0001 |
| 6 | | 1.4779 | 0.9479 | 0.5528 | 0.8988 | 2.5315 | 6.0430 | 6.5025 | 0.0001 |
| 7 | | | | | | 3.0395 | 4.2959 | 5.5666 | 16.7407 |
| 8 | | | | | | 3.5767 | 2.2890 | 2.0125 | 0.0001 |
| 9 | | | | | | 1.0358 | 0.2565 | 0.3716 | 1.0632 |
| 10 | | | | | | | | | 3.3418 |
| 11 | | | | | | | | | 5.0013 |
| 12 | | | | | | | | | 0.7444 |

# S2 The evolution of entropy for extra molecules not presented in the main text.

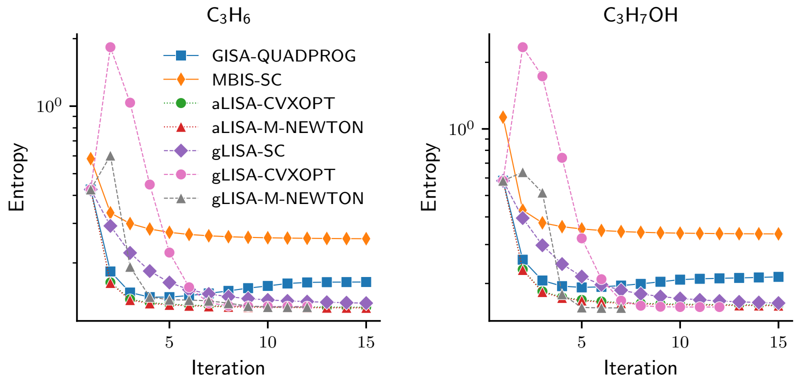

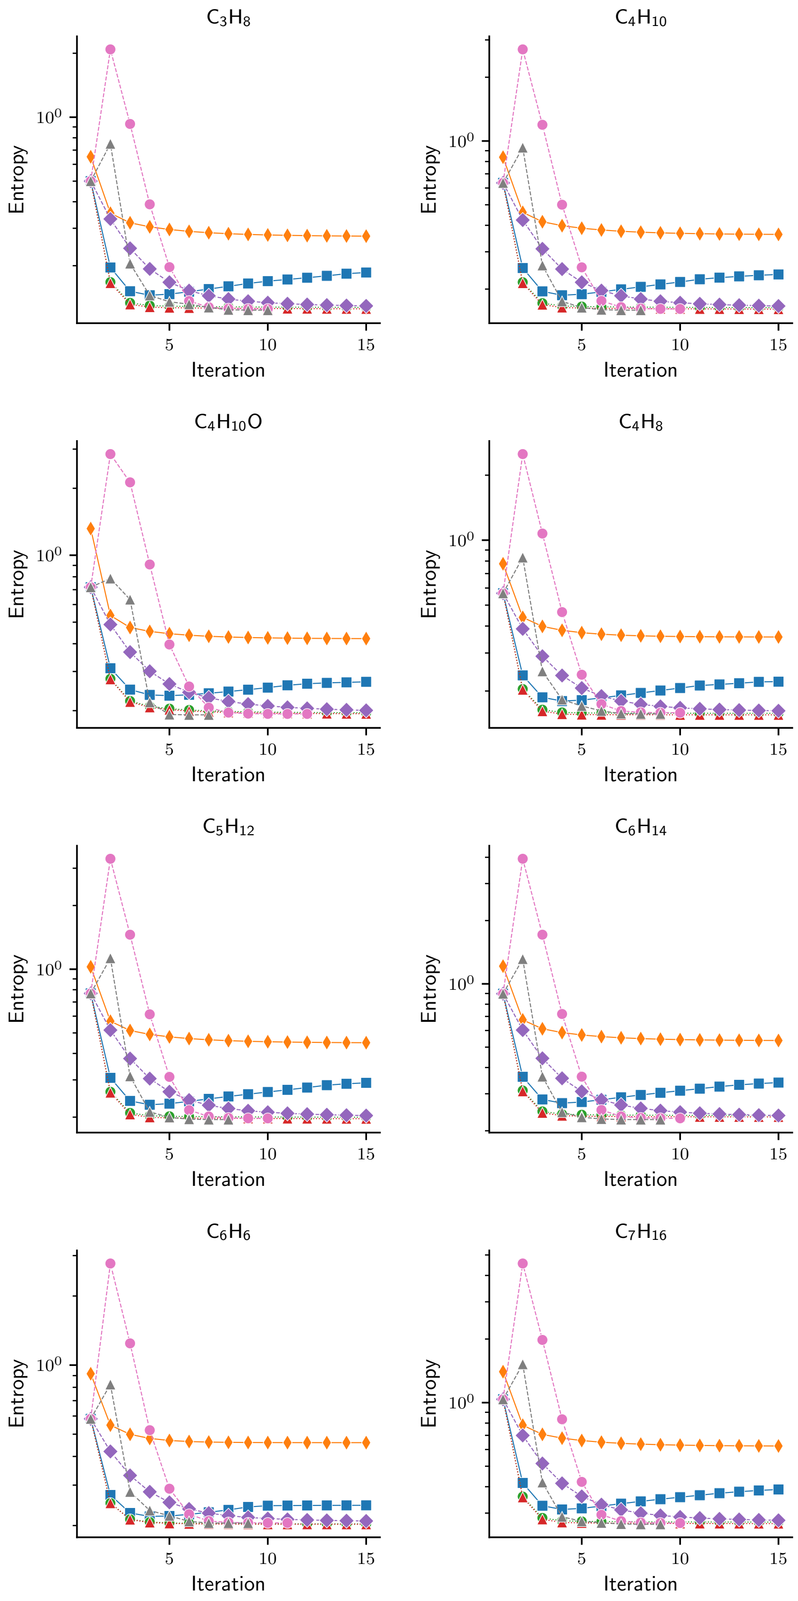
C3H8
C4H10
C4H10O
C4H8
C5H12
C6H14
C6H6
C7H16
Entropy
Iteration
10^0
5
10
15

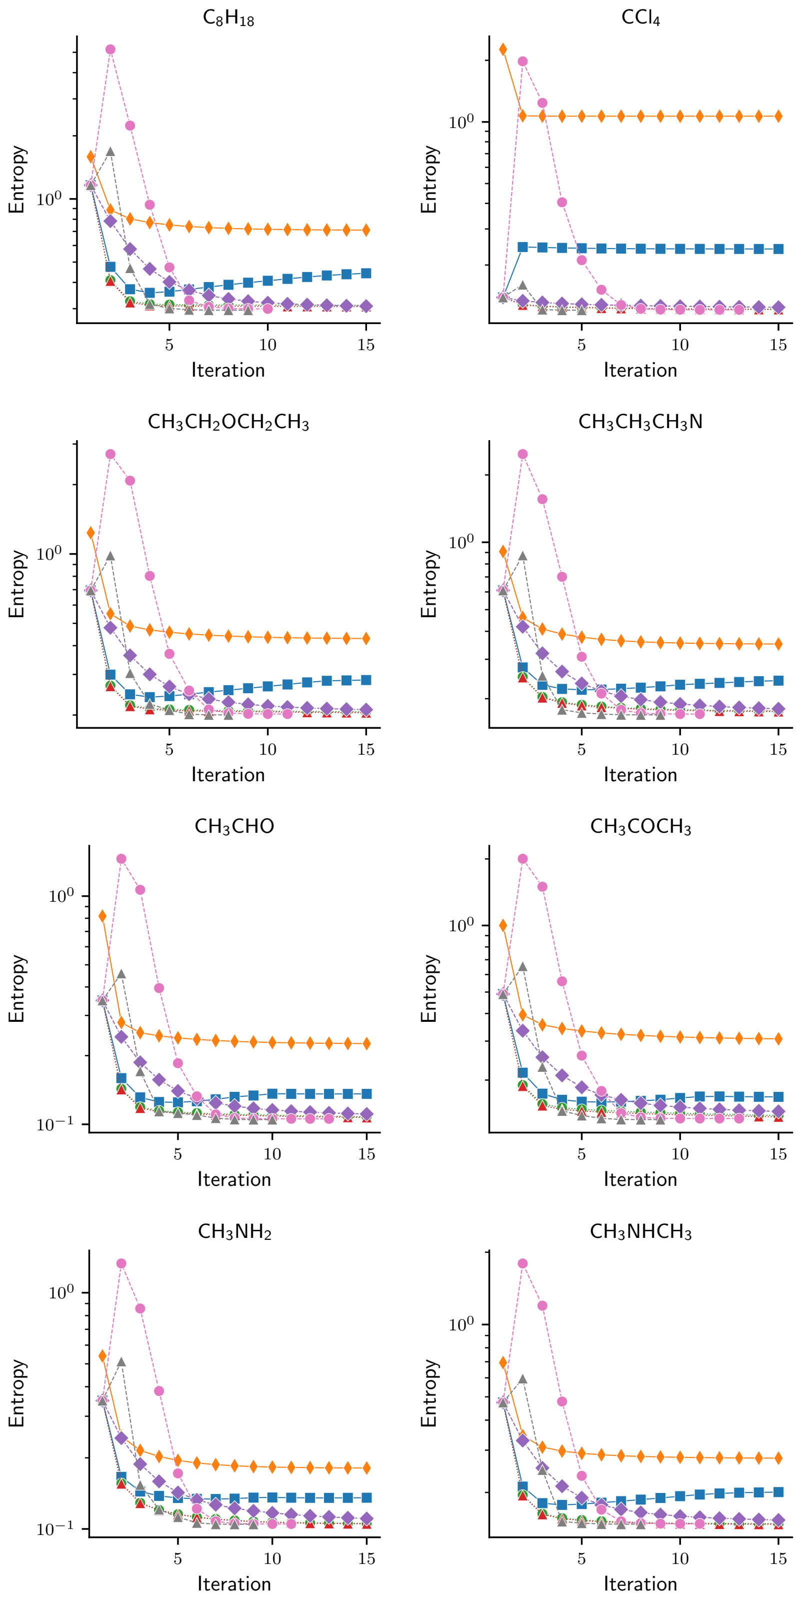

$C_8H_{18}$
$CCl_4$
$CH_3CH_2OCH_2CH_3$
$CH_3CH_3CH_3N$
$CH_3CHO$
$CH_3COCH_3$
$CH_3NH_2$
$CH_3NHCH_3$
Entropy
Iteration
$10^0$
$10^{-1}$
5
10
15

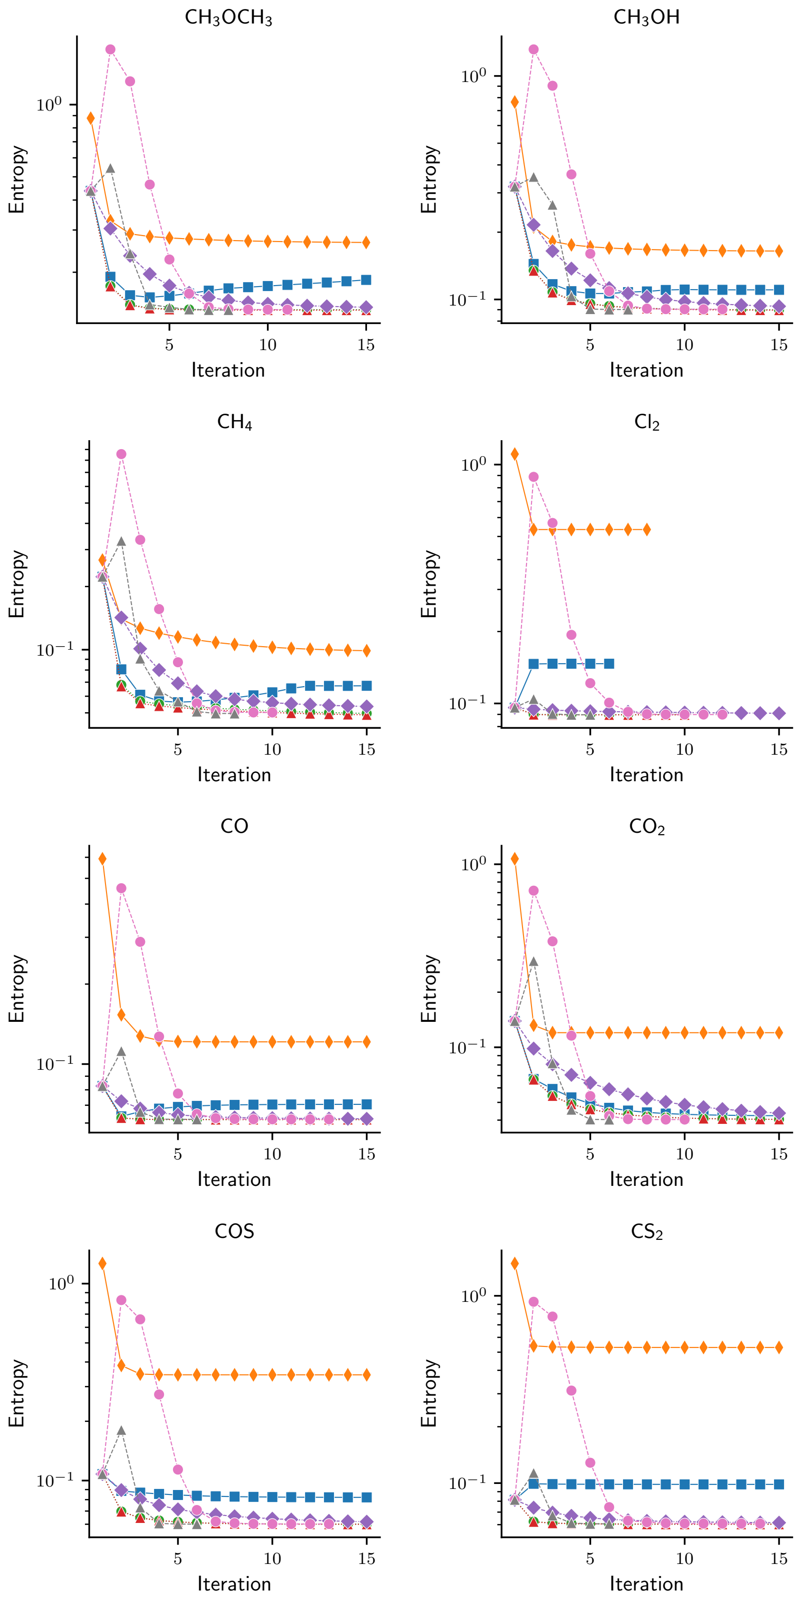

$CH_3OCH_3$
$CH_3OH$
$CH_4$
$Cl_2$
CO
$CO_2$
COS
$CS_2$
Entropy
Iteration
$10^0$
$10^{-1}$
5
10
15

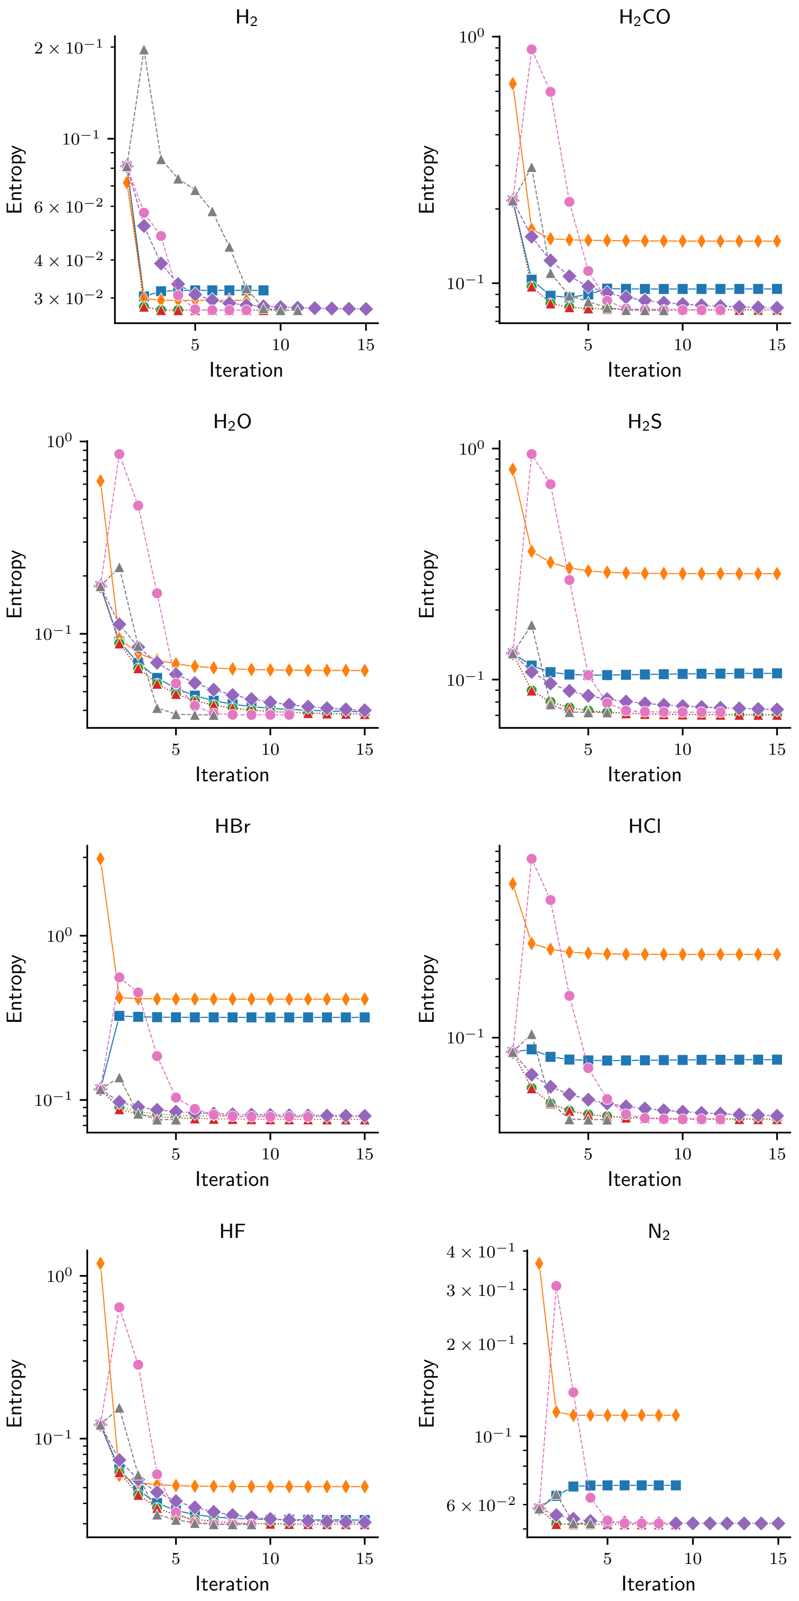

H2
H2CO
H2O
H2S
HBr
HCl
HF
N2
Entropy
Iteration

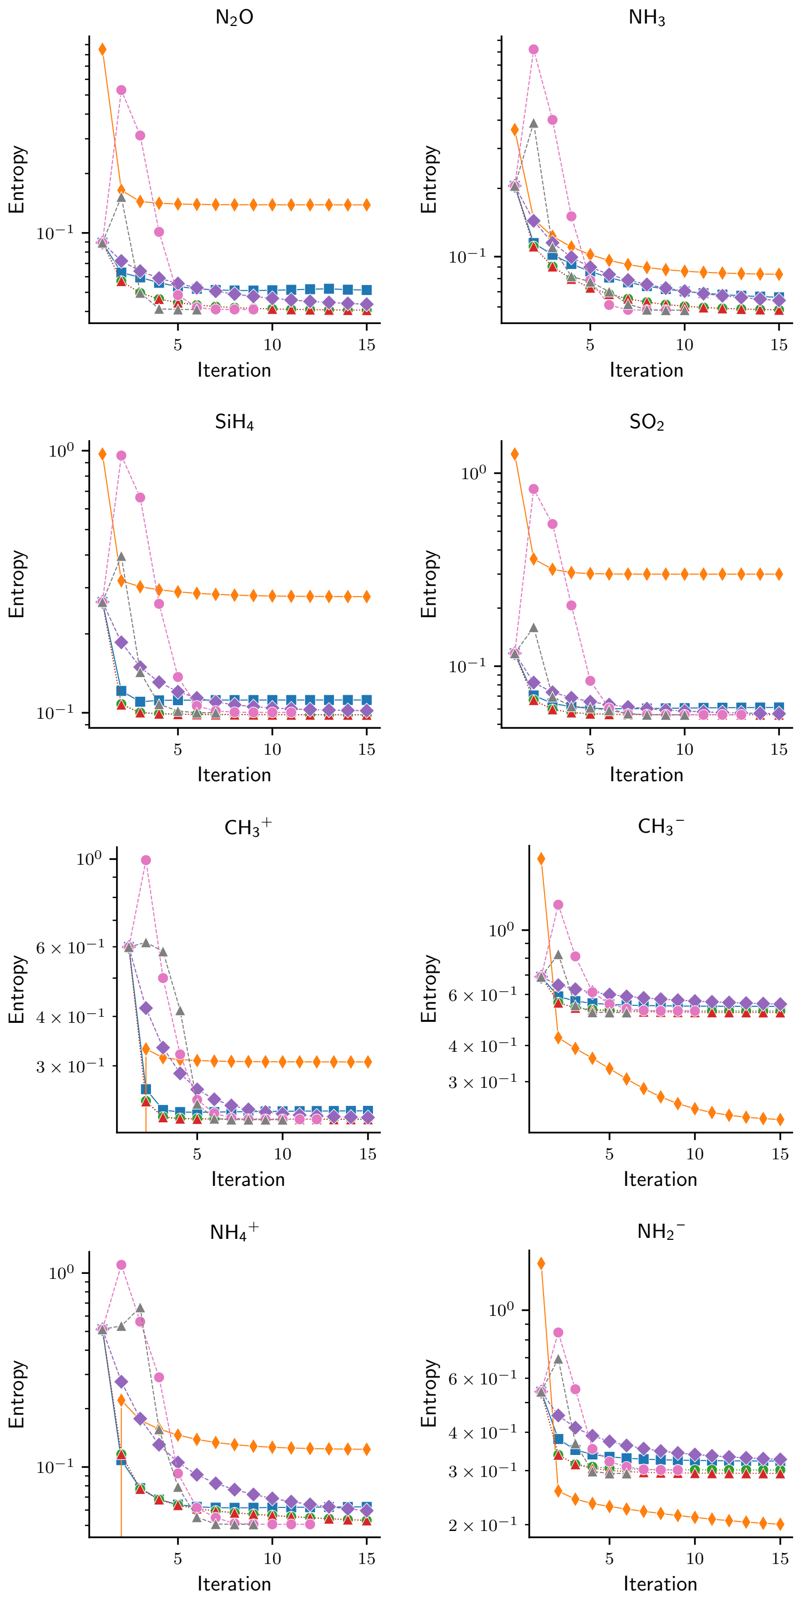
N$_2$O
NH$_3$
SiH$_4$
SO$_2$
CH$_3$$^+$
CH$_3$$^-$
NH$_4$$^+$
NH$_2$$^-$
Entropy
Iteration
$10^{-1}$
$10^{0}$
$6 \times 10^{-1}$
$4 \times 10^{-1}$
$3 \times 10^{-1}$
$2 \times 10^{-1}$
5
10
15

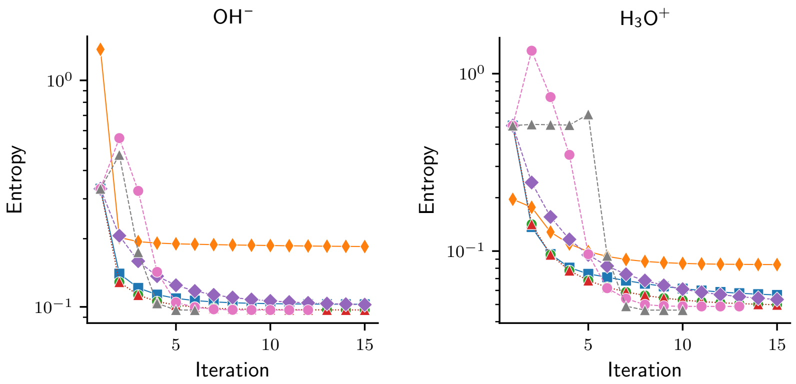

OH⁻
H₃O⁺
Entropy
Iteration
10⁰
10⁻¹
5
10
15
